# Supplementary material for: Formally exact, arbitrarily scalable simulations of exciton dynamics in molecular materials
Source: arXiv:2008.06496 ancillary file (2021-03-12)
Supplement: Supplementary file 1 [file ManuscriptSI__Adaptive_HOPS.pdf]

# Supplementary Information: Formally exact, arbitrarily scalable simulations of exciton dynamics in molecular materials

Leonel Varvelo, Jacob K. Lynd, and Doran I. G. Bennett*
*Department of Chemistry, Southern Methodist University, PO Box 750314, Dallas, TX, USA*

## I. SOURCES OF ERROR

In a HOPS simulation, there are three sources of error for an ensemble averaged property: the statistical error, associated with a finite number of trajectories, the hierarchy error arising from a truncation of the hierarchy, and the time-step error that arises from numerical integration (in this case fourth-order Runge-Kutta).

Here, we characterize the distance between the outcome of two calculations in terms of the mean norm of the population differences on each pigment

$$\sigma = \frac{1}{N_t} \sum_t \sqrt{\frac{1}{2} \sum_n |\vec{P}_n(t) - \vec{p}_n(t)|^2} \tag{1}$$

where the extra factor of $\frac{1}{2}$ ensures $\sigma$ is bounded between 0 and 1.

### A. Number of Trajectories

We estimate the statistical error arising from a finite number of trajectories by bootstrapping [1]. We first calculate $10^4$ trajectories. Then, for each value of $N_{traj}$ we construct $10^4$ ensembles by sampling (with replacement) $N_{traj}$ trajectories from the original ensemble of $10^4$ trajectories. We use the half-width of the 95% confidence interval to characterize the expected error arising from finite sampling. Specifically, we construct a vector ($\vec{\Sigma}_t$) with half-width of the 95% confidence interval for each site population at a given time (t) and estimate the statistical error ($\epsilon$)

$$\epsilon = \frac{1}{\sqrt{2}N_t} \sum_t \left\| \vec{\Sigma}_t \right\| \tag{2}$$

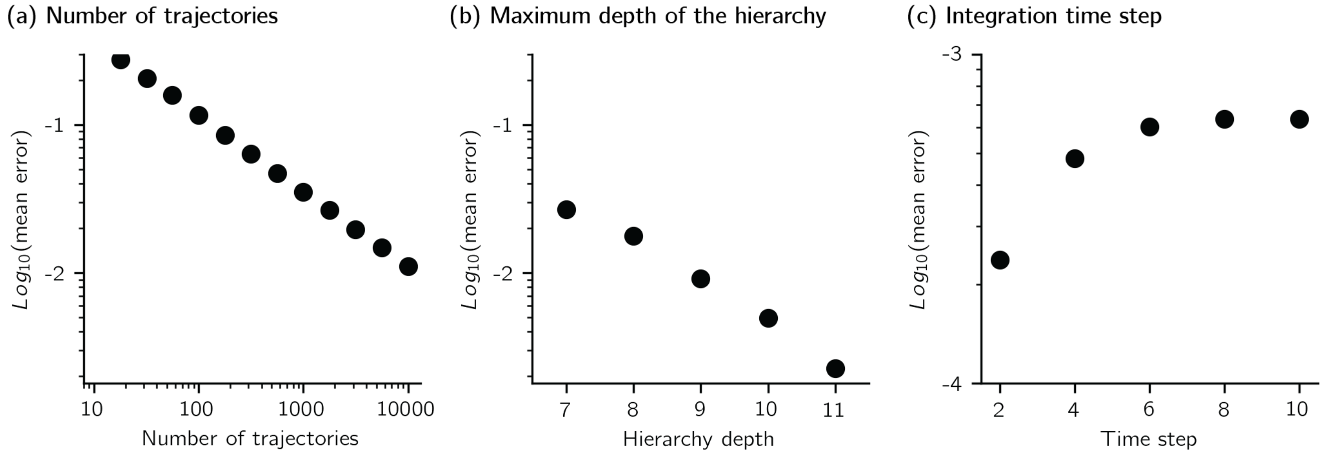


FIG. S1. Comparing error sources in HOPS ensembles. (a) Statistical error from bootstrapping as a function of trajectories with $k_{max} = 10$. (b) Error in population vectors as a function of $k_{max}$ with $N_{\text{traj}} = 10^3$. (c) Error in population vectors as a function of time step with $k_{max} = 10$ and $N_{\text{traj}} = 10^4$. Parameters: V = 50 cm$^{-1}$, $\lambda$ = 50 cm$^{-1}$, $\gamma$ = 50 cm$^{-1}$, and T = 295 K.

* doranb@smu.edu

where the factor of $\sqrt{2}$ ensures consistency with the error definition. Fig. S1a shows the statistical error as a function of number of trajectories.

### B. Depth of the Hierarchy

HOPS calculations are exact for an infinite hierarchy, but numerical calculations require the calculation to consider only auxiliary wave functions up to some maximum depth ($k_{max}$). To isolate the effects of $k_{max}$ on the population vectors, we minimize the influence of statistical error by comparing simulations at different hierarchy depths using the same noise trajectories. We calculate the error at different depths of the hierarchy by comparing the ensemble average population vector to the results when $k_{max} = 12$, using eq. (1). Fig. S1b shows the mean error vs hierarchy depth for $10^3$ trajectories. By $k_{max} = 10$ the hierarchy error is comfortably below 0.01, and we use this value of $k_{max}$ for most of our 5 site calculations.

### C. Time Step

In numerical integration, the time step affects both the accuracy of the trajectory and the computational cost. To test convergence with respect to the time step (dt), we consider matched HOPS trajectories with varying dt values. Figure S1c presents the distribution of mean error (eq. 1) as a function of increasing dt when compared to population vectors calculated using a time step of 1 fs. The error gradually increases as the time step becomes larger. We did not explore the origin of the integration error, though it is notable that the Markovian mode introduces a timescale of decay that is approximately 10 fs. Except where noted otherwise, for the calculations presented here, we have used a time step of 4 fs which is sufficiently short to sample the Markovian dynamics.

### D. Distribution of adaptive error

With the use of an adaptive basis, adHOPS introduces a new form of error into the HOPS framework, arising due to the finite accuracy with which the derivative is calculated at any given time. We calculate the adaptive error for each trajectory in a $10^4$ member ensemble as the mean difference ($\sigma$, eq. (1)) between the equivalent adHOPS and HOPS trajectories. The distribution of adaptive errors (Fig. S2) shows errors spreading more than two orders of magnitude. To explore how error evolves in individual trajectories, we plot the error vs time for trajectories that show extremely high error (red box, red line), moderately high error (green box, green lines), and 'nominal' error behavior (blue box, blue lines). The highest error arises from adHOPS trajectories that diverge from the equivalent HOPS calculations, though these represent around 0.1% of the ensemble. The moderately high errors arise from adHOPS trajectories that show periods in which they drift away from the corresponding HOPS trajectory before returning, as seen by the peak like structure in the error plots. The 'nominal' error of most adHOPS trajectories show small fluctuations in the vicinity of the corresponding HOPS trajectory. We note that the mean adHOPS ensemble population dynamics are even more similar to the corresponding HOPS calculations than these results suggest, due to cancellation of errors. The black line in Fig. S2 shows the error between the ensemble average adHOPS population trajectory compared to the corresponding HOPS ensemble average and has a mean value of $3 \times 10^{-3}$.

## II. CONVERGENCE IN ADHOPS

In an adHOPS calculations we have two convergence parameters that define the hierarchy basis used in our calculations: the maximum depth of the hierarchy ($k_{max}$) and the bound on the derivative error ($\delta$). We explored the possibility of a coupling between these two convergence criteria that would lead to changes in the converged value of one (e.g., $k_{max}$) for different values of the other parameter ($\delta$). Our approach began with a convergence scan for $\delta$ with values, decreasing by logarithmic half-steps (e.g., log($\delta$) = -1, -1.5, -2, etc.), until the difference between two calculations ($\sigma$, eq. (1)) with $\delta$ separated by 1 log unit was less than 0.01. We then ran a convergence scan for $k_{max}$ with values increasing by steps of 1, until the difference between two calculations ($\sigma$, eq. (1)) with $k_{max}$ separated by 2 was less than 0.01. We then ran a new $\delta$ convergence scan at the converged value of $k_{max}$. In all cases we found that this second $\delta$ scan returns the same convergence value as the first, suggesting that the $\delta$ and $k_{max}$ scans are, at least to a first approximation, independent.

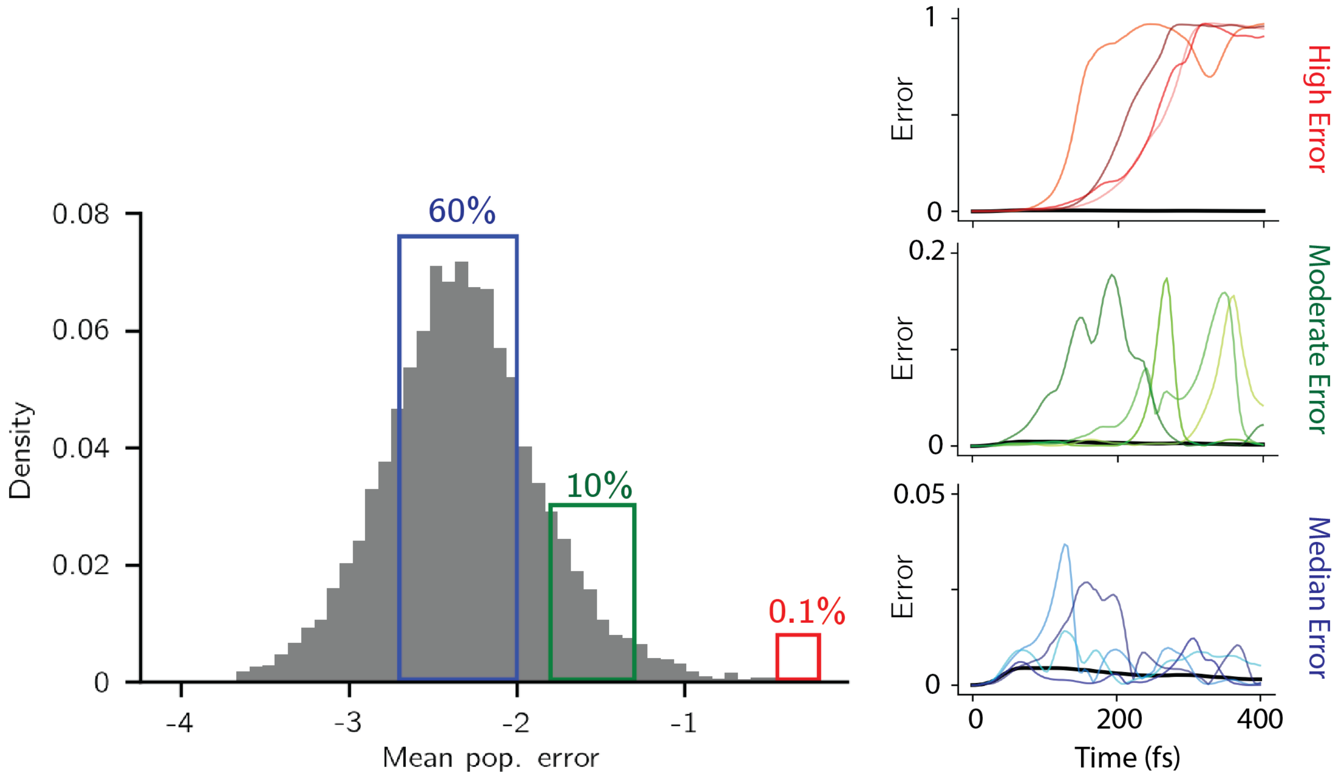


FIG. S2. Population error of individual trajectories and their ensemble distribution. The ensemble contains $10^4$ matched HOPS and adHOPS ($\delta = 10^{-3}$) trajectories. Four trajectories each from median (blue lines), moderate (green lines), and high-error (red lines) subsets of the ensemble are plotted with the ensemble mean (black line). Parameters: V = 50 cm$^{-1}$, $\lambda$ = 50 cm$^{-1}$, $\gamma$ = 50 cm$^{-1}$, T = 295 K, $k_{max}$ = 10, $\delta = 10^{-3}$, $N_{\rm traj} = 10^4$, and dt = 4 fs.

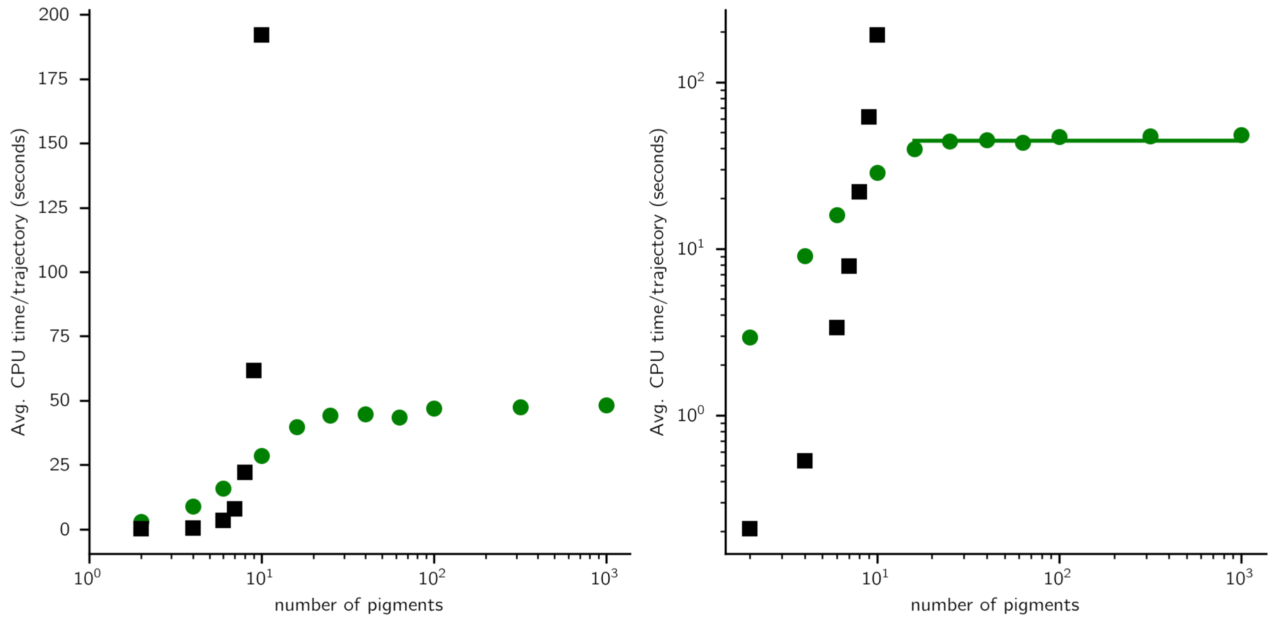


FIG. S3. Average CPU time for running HOPS (black squares) and adHOPS (green circle) simulations. The green line in the right panel shows a linear fit to the data from $N_{pig} = 16$ to 1000, with a coefficient of 0.0277. Calculations were run using Intel Xeon 2.1 GHz processor. Parameters: $V = 50$ cm$^{-1}$, $\lambda = 50$ cm$^{-1}$, $\gamma = 50$ cm$^{-1}$, $T = 295$ K, $k_{max} = 10$, and $\delta = 3 \times 10^{-4}$.

## III. CPU TIMING

In Fig. S3, we compare the CPU time required to run matched HOPS (black squares) and adHOPS (green circles) calculations for the sequence of linear chains presented in Fig. 6 of the main text. We measure the CPU time as the time required to propagate the equation of motion, excluding any time spent in the initial setup. HOPS calculations were only performed for $N_{pig} \leq 10$ due to the extreme computational expense for calculations of larger chains. We find that starting at $N_{pig} = 9$, adHOPS calculations require less CPU time per trajectory than the matches HOPS calculations. Further increasing the size of the linear chain rapidly leads to HOPS calculations that are unwieldy. On the other hand, adHOPS calculations including $10^3$ pigments can be performed conveniently.

Using the log-log plot for CPU time vs system size (right panel) we determine a residual scaling of $O(N_{pig}^{0.03})$ for the adHOPS calculations in the size-invariant region. This results in a 20% increase in CPU time per trajectory when increasing the linear chain length from $N_{pig} = 16$ to 1000. We have not yet identified the origin of the residual scaling.

## IV. CODE

With the exception of the SI section on CPU timing (above), all calculations presented here used the version 1.00 of MesoHOPS. The CPU timing section used version 1.10 of MesoHOPS, which is also the version archived with Zenodo. The changes in the code do not influence any conclusions though numerical differences may be observed resulting from changes in the code structure to improve numerical performance of the adaptive algorithm.

MesoHOPS V1.1.0: http://doi.org/10.5281/zenodo.4592583

MesoHOPS V1.0.0: (https://github.com/MesoscienceLab/mesohops, commit: 86e991917c9e57d63dfc9b5e140d1f6112544f98)

## REFERENCES

[1] A. C. Davison and D. V. Hinkley. *Bootstrap Methods and their Application*. Cambridge Series in Statistical and Probabilistic Mathematics. Cambridge: Cambridge University Press, 1997. ISBN: 978-0-521-57471-6. DOI: `10.1017/CBO9780511802843`. URL: `https://www.cambridge.org/core/books/bootstrap-methods-and-their-application/ED2FD043579F27952363566DC09CBD6A`.
